# Supplementary material for: Reinforcement Learning-based Automatic Diagnosis of Acute Appendicitis in Abdominal CT
Source: arXiv:1909.00617 source file (2019-09-02)
Supplement: Supplementary file 1 [file patch_size.tex]

\documentclass[crop,tikz]{standalone}% 'crop' is the default for v1.0, before it was 'preview'
%\usetikzlibrary{...}% tikz package already loaded by 'tikz' option
\usepackage{pgfplots}
\usepackage{amsmath}
\begin{document}
\begin{tikzpicture}
\tikzstyle{every node}=[font=\normalsize]
\begin{axis}[
	symbolic x coords = {
		$75$,
		$150$, 
		$225$, 
		$300$, 
	},
	xtick = data,
	%x tick label style={rotate=90, anchor=east},
	xlabel = Edge length of the input patch ($\text{voxel}$),
	y label style={at={(axis description cs:0.08,0.5)},anchor=south},
	ylabel = Mean AUC,
	ymax = 1.0,
	]
	\addplot[ybar, bar width = 20, fill=blue, 
	nodes near coords={\pgfmathprintnumber[fixed zerofill, precision=3]{\pgfplotspointmeta}},]
		coordinates{
		($75$, 0.952)
		($150$, 0.790)
		($225$, 0.722)
		($300$, 0.712)
		
	};	

\end{axis}
\end{tikzpicture}
\end{document}
