# Supplementary material for: Reinforcement Learning-based Automatic Diagnosis of Acute Appendicitis in Abdominal CT
Source: arXiv:1909.00617 source file (2019-09-02)
Supplement: Supplementary file 2 [file sampletikz.tex]

\documentclass[crop,tikz]{standalone}% 'crop' is the default for v1.0, before it was 'preview'
%\usetikzlibrary{...}% tikz package already loaded by 'tikz' option
\begin{document}
\begin{tikzpicture}
  \draw (0,0) -- (10,10); % ...
\end{tikzpicture}
\end{document}
