# Supplementary material for: Reinforcement Learning-based Automatic Diagnosis of Acute Appendicitis in Abdominal CT
Source: arXiv:1909.00617 source file (2019-09-02)
Supplement: Supplementary file 4 [file sample_line_plot.tex]

\documentclass[crop,tikz]{standalone}% 'crop' is the default for v1.0, before it was 'preview'
%\usetikzlibrary{...}% tikz package already loaded by 'tikz' option
\usepackage{pgfplots}
\begin{document}
\begin{tikzpicture}
	\tikzstyle{every node}=[font=\small]
  \begin{axis}[
	x label style={at={(axis description cs:0.5,0.0)},anchor=north},
    y label style={at={(axis description cs:0.1,.5)},anchor=south},  
    %title={RTW with too small step length},
     %x label style={at={(axis description cs:0.5,0.0)},anchor=north},
    %y label style={at={(axis description cs:0.1,.5)},anchor=south},     
    xlabel={Training samples (\%)},
    ylabel={AV landmark localization error (mm)},    
    xmin=65, xmax=310,
    ymin=0.5, ymax=1.2,
    xtick={ 75,150,300},
    ytick={0.6,1},
    legend pos=north east,
   % ymajorgrids=true,
    %grid style=dashed,
]
   
    
\addplot[color=blue, mark=triangle*]
coordinates{(75, 0.961) (150, 0.7904) (300, 0.7124)};
	\label{plot_three}    
    %\addlegendentry{DQN}


\end{axis}
\end{tikzpicture}
\end{document}
